# Supplementary material for: Self-Diagnosing GAN: Diagnosing Underrepresented Samples in Generative Adversarial Networks
Source: arXiv:2102.12033 source file (2021-10-26)
Supplement: Supplementary file 7 [file color_mnist_supp.tex]

\begin{figure}[!ht]
    \centering
    \subfloat[Baseline rate 99\%]{\includegraphics[width=0.2\linewidth]{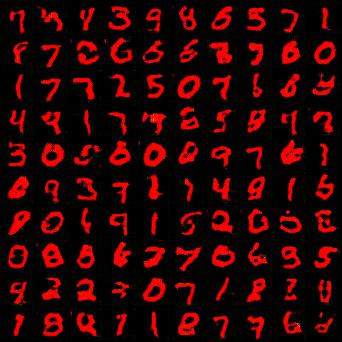}} \quad
    \subfloat[Baseline rate 95\%]{\includegraphics[width=0.2\linewidth]{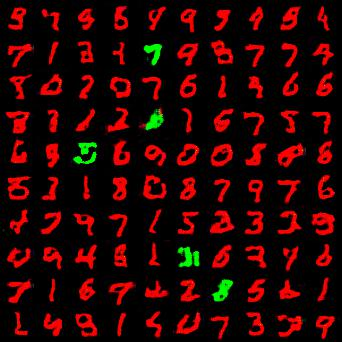}}\quad
    \subfloat[Baseline rate 90\%]{\includegraphics[width=0.2\linewidth]{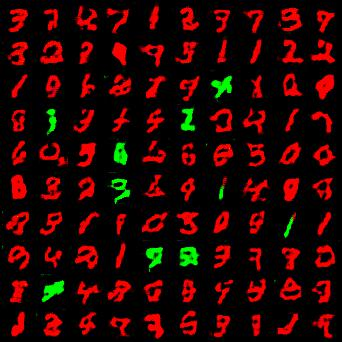}} \\
    \subfloat[GOLD rate 99\%]{\includegraphics[width=0.2\linewidth]{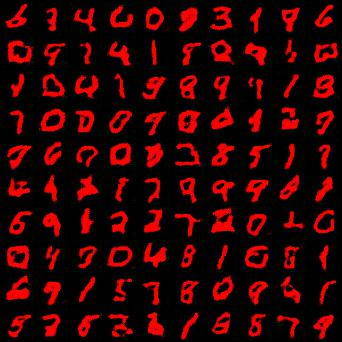}} \quad
    \subfloat[GOLD rate 95\%]{\includegraphics[width=0.2\linewidth]{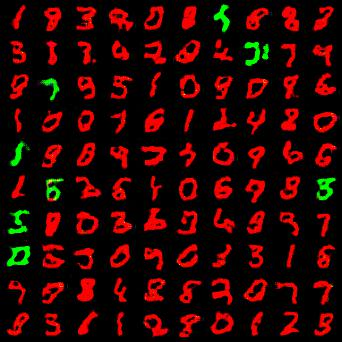}}\quad
    \subfloat[GOLD rate 90\%]{\includegraphics[width=0.2\linewidth]{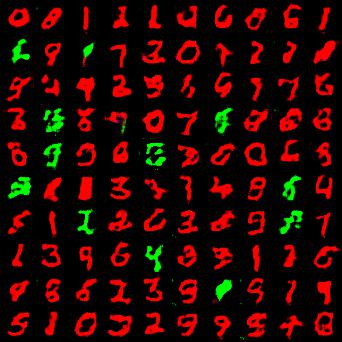}} \\
    \subfloat[Top-k rate 99\%]{\includegraphics[width=0.2\linewidth]{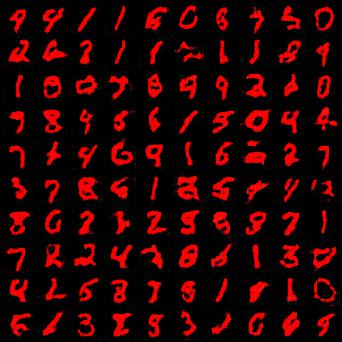}} \quad
    \subfloat[Top-k rate 95\%]{\includegraphics[width=0.2\linewidth]{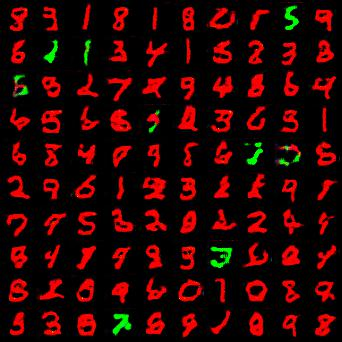}}\quad
    \subfloat[Top-k rate 90\%]{\includegraphics[width=0.2\linewidth]{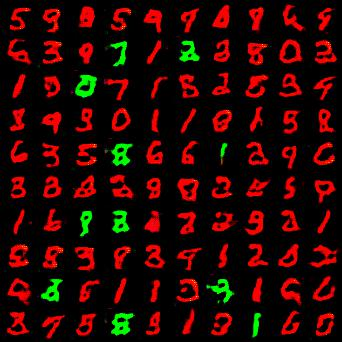}}\\
    \subfloat[PacGAN rate 99\%]{\includegraphics[width=0.2\linewidth]{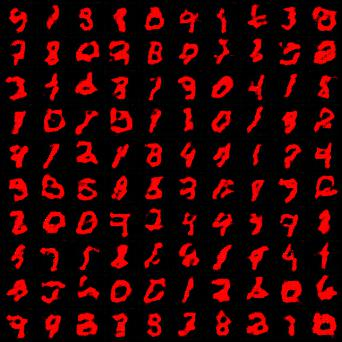}} \quad
    \subfloat[PacGAN rate 95\%]{\includegraphics[width=0.2\linewidth]{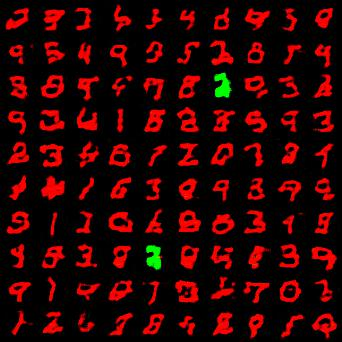}} \quad
    \subfloat[PacGAN rate 90\%]{\includegraphics[width=0.2\linewidth]{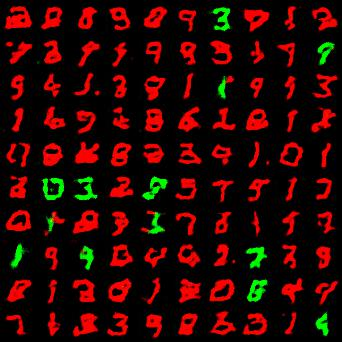}} \\
    \subfloat[Ours rate 99\%]{\includegraphics[width=0.2\linewidth]{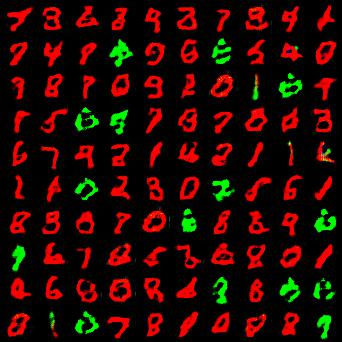}} \quad
    \subfloat[Ours rate 95\%]{\includegraphics[width=0.2\linewidth]{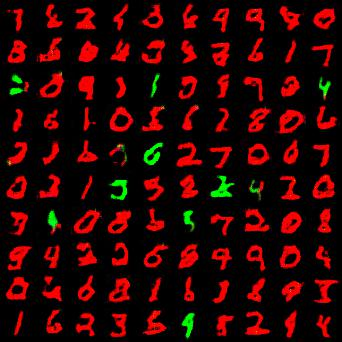}}\quad
    \subfloat[Ours rate 90\%]{\includegraphics[width=0.2\linewidth]{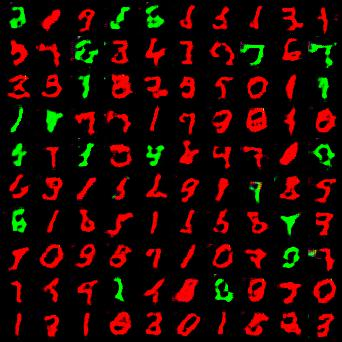}} \\
    \caption{Colored MNIST generated samples of various GANs on different majority rate.}
    \label{fig:color-mnist-supp}
\end{figure}
