# Supplementary material for: Self-Diagnosing GAN: Diagnosing Underrepresented Samples in Generative Adversarial Networks
Source: arXiv:2102.12033 source file (2021-10-26)
Supplement: Supplementary file 13 [file controlled_re_appendix.tex]

\begin{table}[!tb]
\centering
\caption{Reconstruction Error (RE) score of green training samples in Colored MNIST and FMNIST samples in a mixture of MNIST and FMNIST on different majority rate $\rho$.}
\label{table:controlled_recon_appendix}
\vspace{0.2em}
\begin{tabular}{c|ccc|ccc}
\toprule
Dataset & \multicolumn{3}{c|}{Colored MNIST} & \multicolumn{3}{c}{MNIST-FMNIST}\\
\midrule
Majority rate $\rho$ &{99\%} &{95\%} &{90\%}  &{99\%} &{95\%} &{90\%}\\
\midrule
% Baseline & 0 & 680.46 & 70.5 & 53.73 & 64.09 & 47.48 \\
% GOLD~\cite{GOLD} & 0 & 678.83 & & 46.83 & & 47.78 \\
% Top-k~\cite{sinha2020top} & 0 & 681.42 & & 53.47 & & 51.28 \\
% PacGAN~\cite{lin2020pacgan} & 0 & 677.24 & & 55.66 & & 44.02 \\
% Inclusive GAN~\cite{InclusiveGAN} & 0 & 679.79 & & 52.71 && \textbf{34.89} \\
Vanilla & 0.838\scriptsize{$\pm$0.033}  & 0.236\scriptsize{$\pm$0.037}  & 0.218\scriptsize{$\pm$0.058}& 0.290\scriptsize{$\pm$0.019}& 0.227\scriptsize{$\pm$0.001}& 0.215\scriptsize{$\pm$0.010}\\
GOLD  & 0.813\scriptsize{$\pm$0.002}& 0.297\scriptsize{$\pm$0.146}& 0.200\scriptsize{$\pm$0.022}& 0.296\scriptsize{$\pm$0.008} & 0.241\scriptsize{$\pm$0.005} & 0.218\scriptsize{$\pm$0.004}\\
Top-k  & 0.831\scriptsize{$\pm$0.022}& 0.210\scriptsize{$\pm$0.012} & 0.223\scriptsize{$\pm$0.015}& 0.281\scriptsize{$\pm$0.012} & 0.232\scriptsize{$\pm$0.006}& 0.221\scriptsize{$\pm$0.007}\\
PacGAN  & 0.810\scriptsize{$\pm$0.001}  & 0.244\scriptsize{$\pm$0.005} & 0.233\scriptsize{$\pm$0.052}& 0.313\scriptsize{$\pm$0.026} & 0.251\scriptsize{$\pm$0.013}& 0.225\scriptsize{$\pm$0.007}\\
Inclusive GAN & 0.812\scriptsize{$\pm$0.001} & 0.274\scriptsize{$\pm$0.060}& 0.216\scriptsize{$\pm$0.024}& 0.283\scriptsize{$\pm$0.012} & 0.230\scriptsize{$\pm$0.015} & 0.220\scriptsize{$\pm$0.011}\\
\textbf{Dia-GAN}  & \textbf{0.224\scriptsize{$\pm$0.020}}&  \textbf{0.204\scriptsize{$\pm$0.018}} & \textbf{0.197\scriptsize{$\pm$0.026}} & \textbf{0.264\scriptsize{$\pm$0.007}} & \textbf{0.219\scriptsize{$\pm$0.016}} & \textbf{0.206\scriptsize{$\pm$0.002}}\\
\bottomrule
\end{tabular}
\end{table}
