# Supplementary material for: Self-Diagnosing GAN: Diagnosing Underrepresented Samples in Generative Adversarial Networks
Source: arXiv:2102.12033 source file (2021-10-26)
Supplement: Supplementary file 15 [file hingegan_appendix.tex]

\begin{table}[t]
\caption{(Details of Table~\ref{table:hingegan}) HingeGAN on CIFAR-10 and CelebA.}
\label{table:hingegan_appendix}
\vspace{0.2em}
\centering
\begin{tabular}{c|cc|c}
\toprule
\multirow{2}{*}{}     &  \multicolumn{2}{c|}{CIFAR-10} & CelebA\\
\cmidrule{2-4}
& FID $\downarrow$ & IS $\uparrow$ & FID $\downarrow$\\
\midrule
HingeGAN & 21.99\scriptsize{$\pm$1.73} & 7.67\scriptsize{$\pm$0.16} & 6.66\scriptsize{$\pm$0.06}\\
\textbf{Dia-HingeGAN} & \textbf{18.74\scriptsize{$\pm$1.79} }   & \textbf{8.02\scriptsize{$\pm$0.14}} & \textbf{5.98\scriptsize{$\pm$0.15}}\\
\bottomrule
\end{tabular}
\end{table}
