# Supplementary material for: Self-Diagnosing GAN: Diagnosing Underrepresented Samples in Generative Adversarial Networks
Source: arXiv:2102.12033 source file (2021-10-26)
Supplement: Supplementary file 17 [file stylegan_appendix.tex]

\begin{table}[h]
%\caption{Global caption}
\caption{(Details of Table~\ref{tab:stylegan2}) StyleGAN2 on FFHQ 256x256.}
\label{tab:stylegan2_appendix}
\vspace{0.2em}
\centering
\begin{tabular}{c|ccc}
    \toprule
        %& StyleGAN2 & \textbf{Dia-StyleGAN2}  \\
        %\midrule
        %FID $\downarrow$ & 14.07 & \textbf{11.89} \\
        & FID $\downarrow$ & P $\uparrow$   & R $\uparrow$ \\
        \midrule
        StyleGAN2 & 14.07\scriptsize{$\pm$3.07}   & \textbf{0.72\scriptsize{$\pm$0.02}}  & 0.27\scriptsize{$\pm$0.03} \\
        GOLD    & 15.53\scriptsize{$\pm$4.14} & 0.69\scriptsize{$\pm$0.00}  & 0.29\scriptsize{$\pm$0.02} \\
        \textbf{Dia-StyleGAN2}  & \textbf{11.89\scriptsize{$\pm$0.21}} & 0.69\scriptsize{$\pm$0.01}  & \textbf{0.30\scriptsize{$\pm$0.01}} \\
        \bottomrule
\end{tabular}
\end{table}
